# Supplementary material for: A Bayesian Non-parametric Approach for Causal Mediation with a Post-treatment Confounder
Source: arXiv:2305.05017 source file (2023-05-08)
Supplement: Supplementary file 2 [file tableEDP_real_avg_supp2.tex]

\begin{table}[htbp] %[p]
    % \fontsize{11}{11}\selectfont
    \caption{\label{EDPM:tab:avgsupp2} Posterior means (95\% credible intervals) of NIE, NDE, and ATE under the standard ignorability assumption without a post-treatment confounder.}
    \centering
        \begin{tabular}[htp]{c|rrr} %[htbp]
        \toprule
        \multicolumn{1}{c}{CE} & \multicolumn{1}{c}{Est.} & \multicolumn{2}{c}{95\% CI} \\
        
        \midrule
        NIE & -0.09 & -0.66 &  0.37 \\
        NDE & -3.08 & -4.83 & -1.49 \\
        ATE & -3.17 & -4.83 & -1.61 \\
        \bottomrule

    \end{tabular}
\end{table}
